# Supplementary material for: "When He Feels Cold, He Goes to the Seahorse"-Blending Generative AI into Multimaterial Storymaking for Family Expressive Arts Therapy
Source: arXiv:2402.06472 source file (2024-02-09)
Supplement: Supplementary file 1 [file 9-appendix.tex]

\section{Appendix}
\clearpage
\begin{figure*}[ht]
  \centering
  \includegraphics[width=0.6\linewidth]{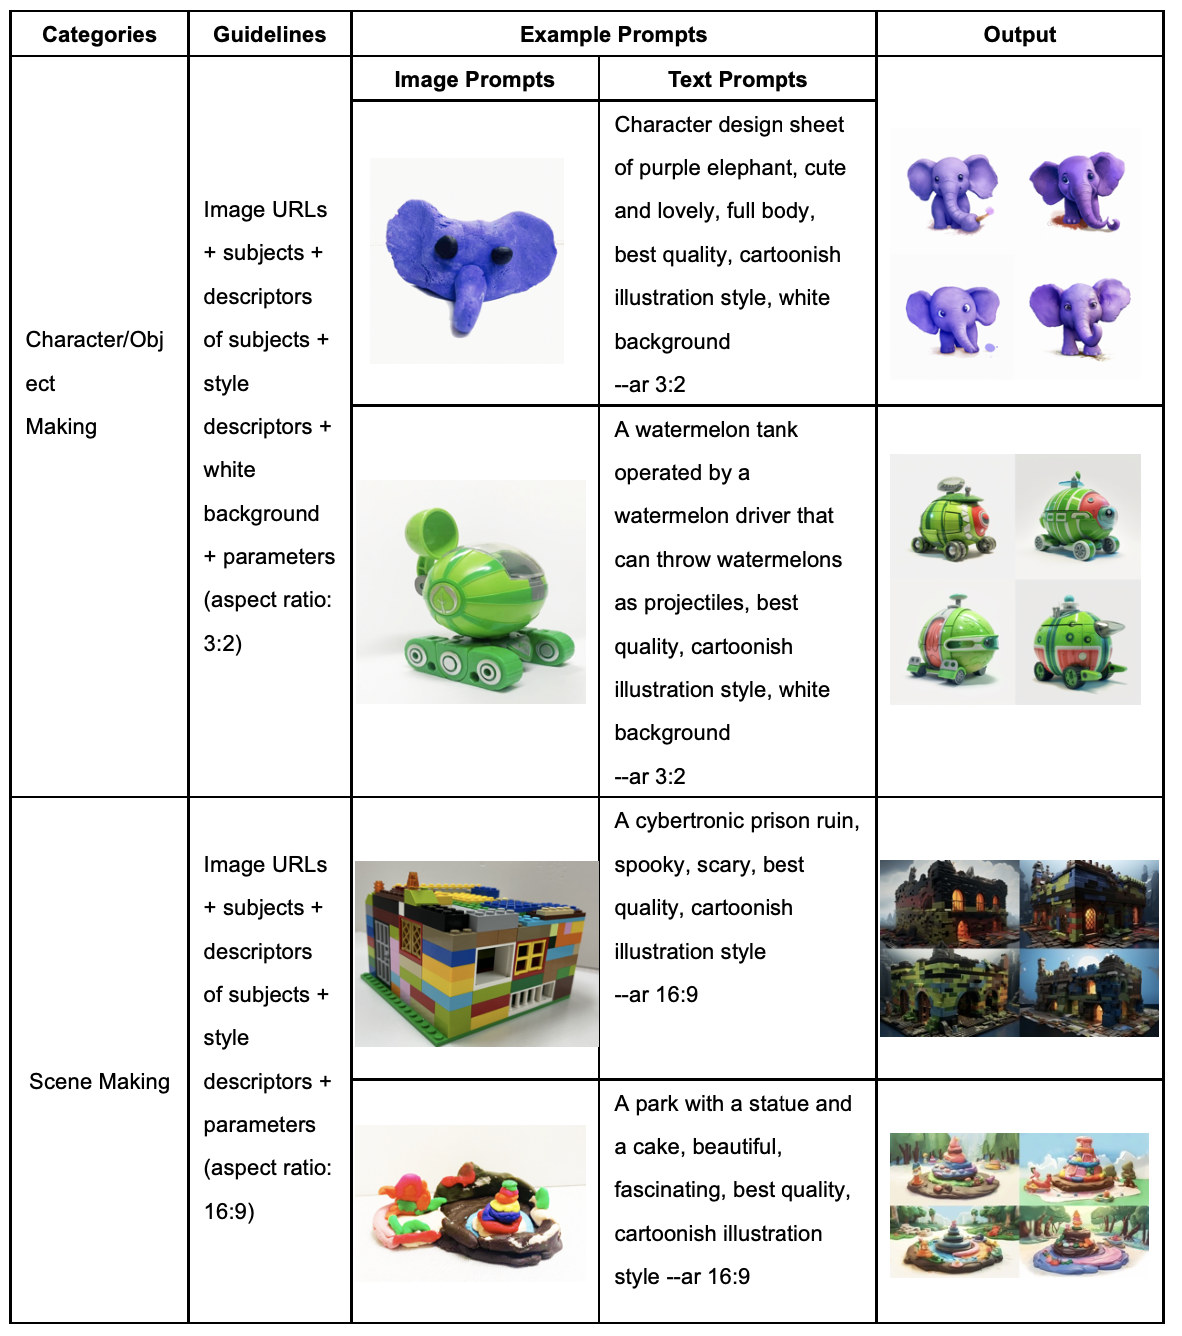} % 用实际的图片文件名替换 example-image-a
  \vspace{8mm}
  \caption{Guidelines and Examples on Midjourney Prompts}
  \label{fig:appendix_a_image}
\end{figure*}

\begin{figure*}[ht]
  \centering
  \includegraphics[width=0.5\linewidth]{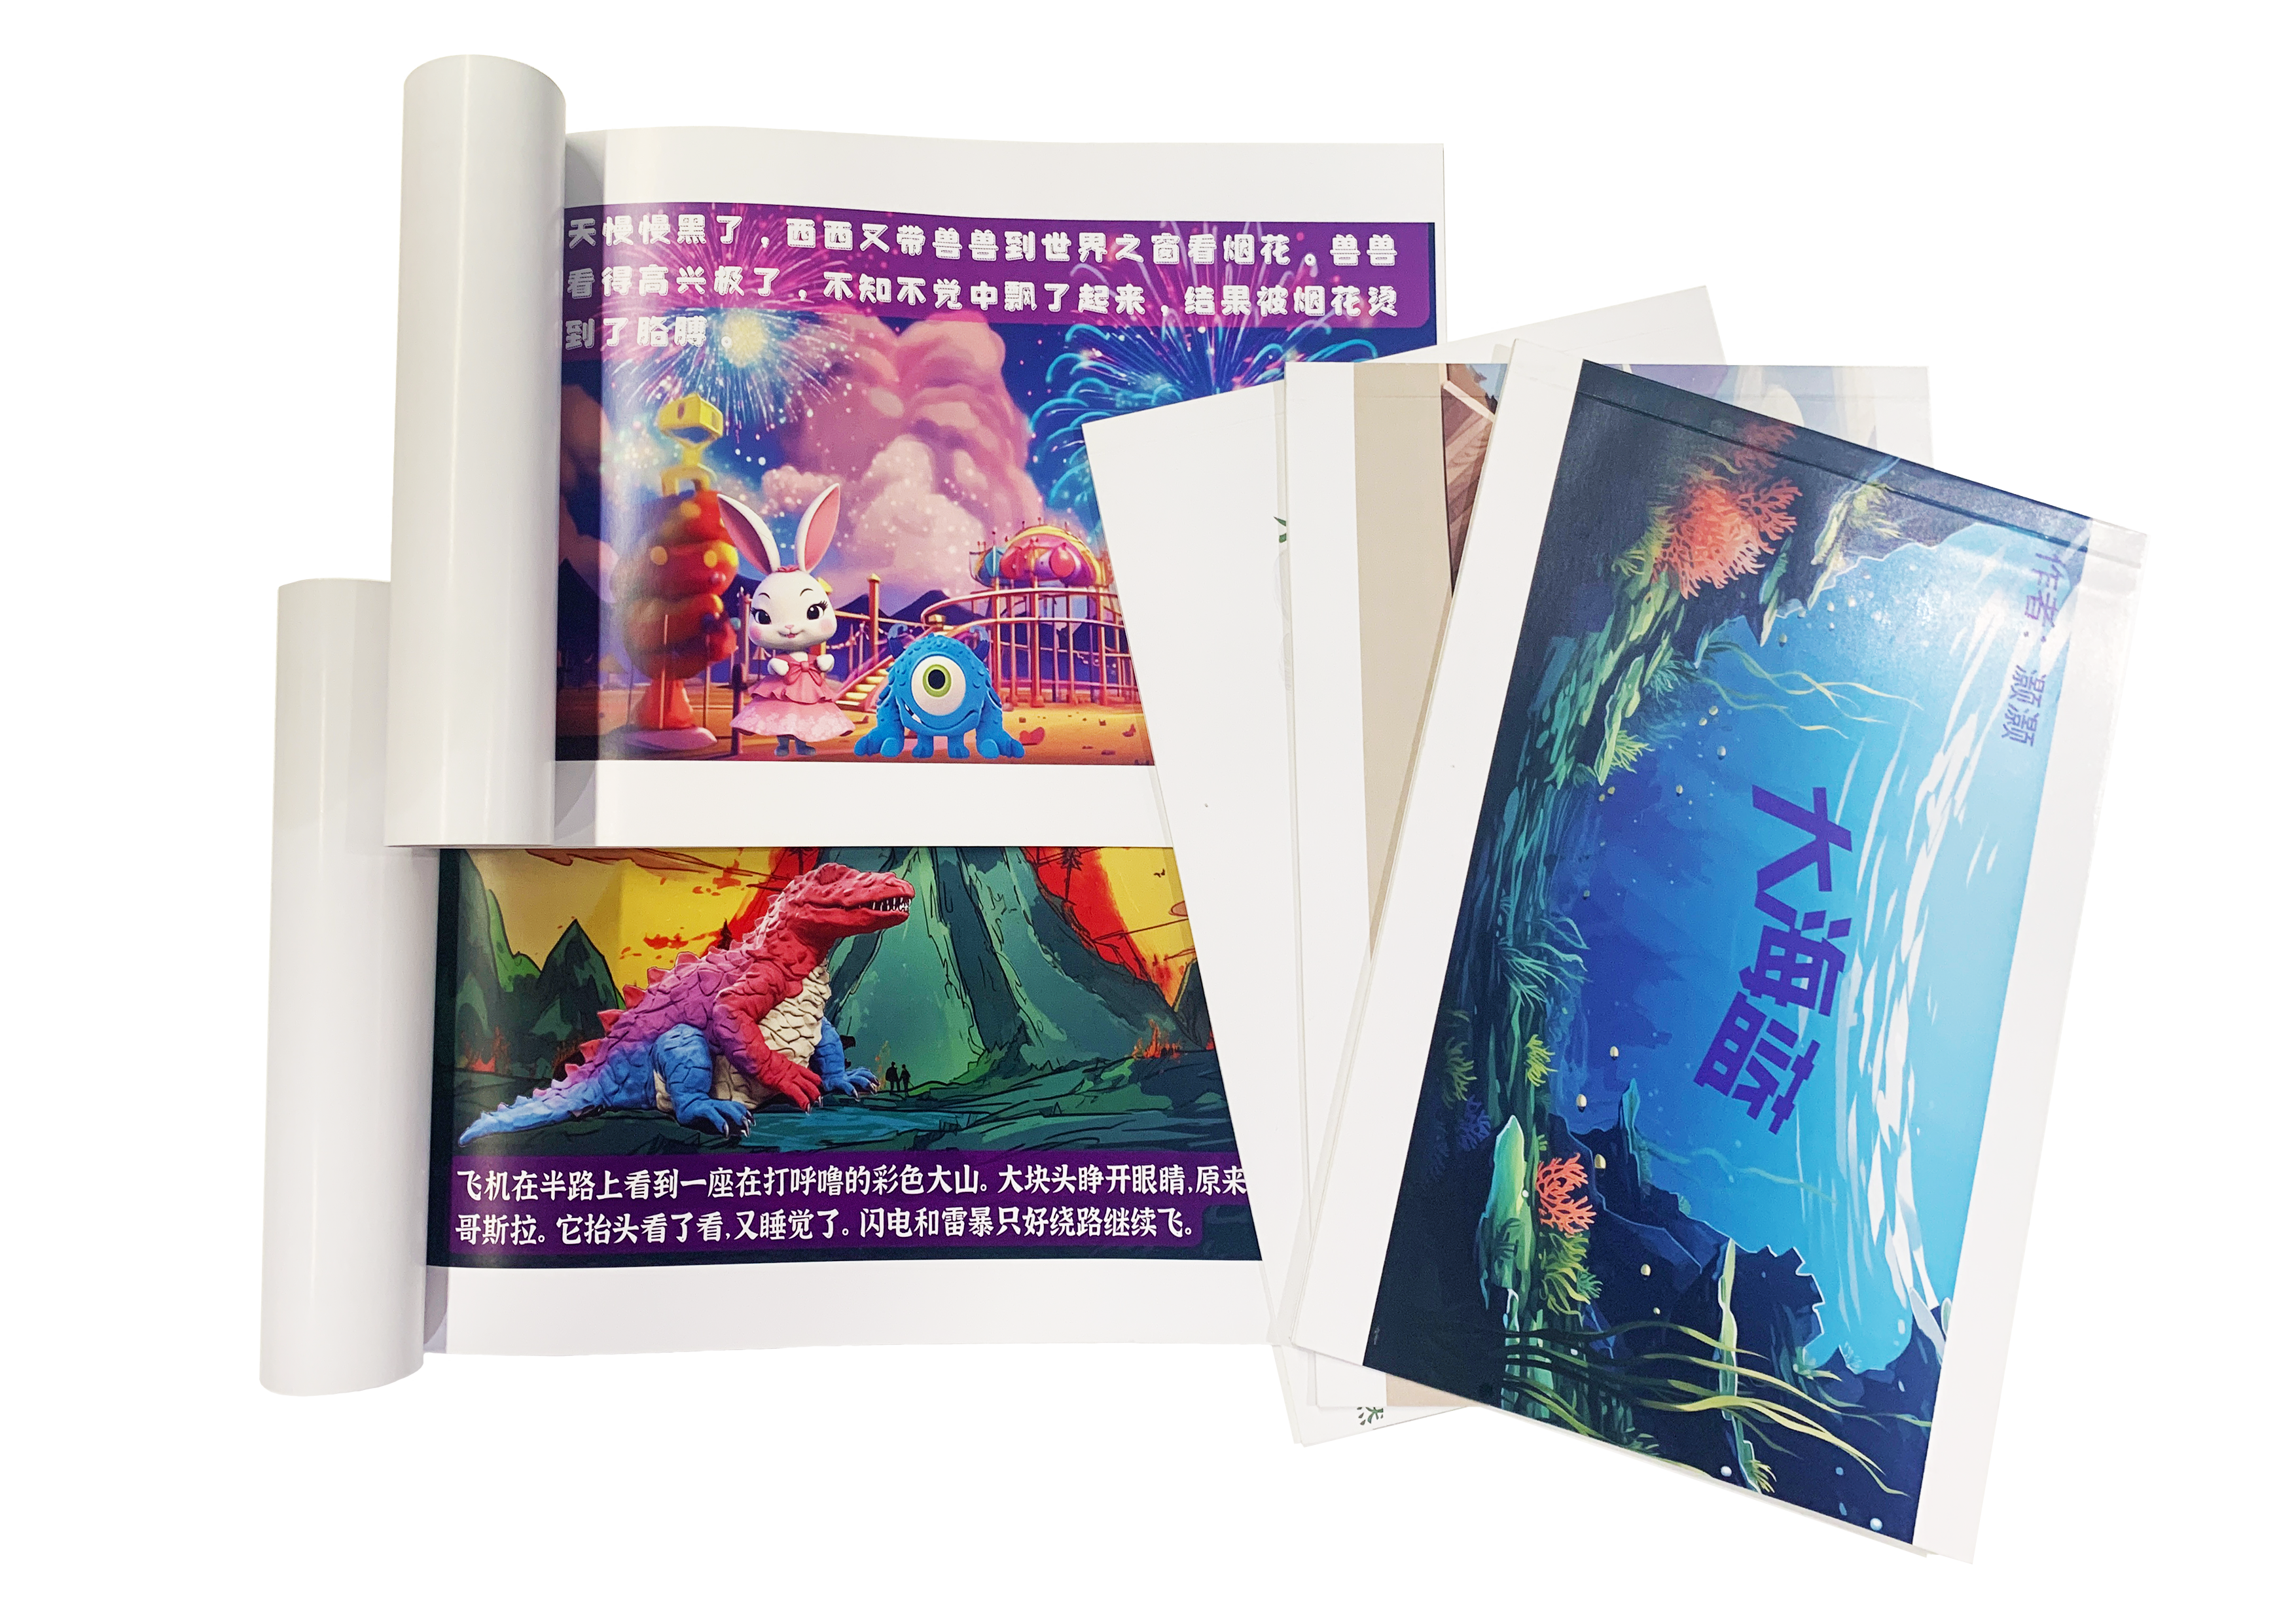} % 用实际的图片文件名替换 example-image-a
  \vspace{-4mm}
  \caption{The Visual Presentation of Physical Storybooks Printed for Families}
  \label{fig:appendix_a_image}
  \Description{Figure 7 shows a physical storybook created by a family using generative AI. T1 and researchers used retouching tools based on the handmade multimaterial storybook frames.}
\end{figure*}

\begin{table*}[ht]
\caption{Summary of the Needs from Children, Parents, and Therapists.}
\centering
\label{tab:finding1need}
\small

\begin{tabular}{|>{\centering\arraybackslash}m{1.5cm}|>{\raggedright\arraybackslash}m{3.5cm}|m{7.5cm}|}
\hline
\textbf{Roles} & \textbf{Needs} & \textbf{Description} \\
\hline
\multirow{5}{*}{Children}
& Diverse Material for Creative Exploration and Expression
& 
\begin{itemize}[label=--]
\item Offering diverse materials can benefit children's self-regulation and motor skills; 
\item Enrich children's non-verbal expression;;
\item Promise huge creative empowerment.
\end{itemize}  
\\
\cline{2-3}
& Personal Relevance
& 
\begin{itemize}[label=--]
\item Integrating themselves or their family members into their stories; 
\item Personal toys were also integrated into their stories.
\end{itemize}   
\\
\cline{2-3}
& Sense of Accomplishment
&
\begin{itemize}[label=--]
\item Artifacts co-created with AI exceeded children's expectations; 
\item Sharing their own storybooks with family members or their peers.
\end{itemize}
\\
\cline{2-3}
& Renarration and Recreation beyond the Therapeutic Sessions
&
\begin{itemize}[label=--]
\item Many children took the AI-generated materials home and continued making new stories at home.
\end{itemize}
\\
\hline
\multirow{4}{*}{Parents}
& Discovering New Aspects of Children
& 
\begin{itemize}[label=--]
\item The artifacts and process of their family storymaking helped uncover children's demands for parents;
\item Parents discovered children's less noticeable life experiences through connecting stories and life;
\end{itemize}  
\\
\cline{2-3}
& Reflection in Therapeutic Storymaking
& 
\begin{itemize}[label=--]
\item Some parents meaningfully reflected on their roles and their family interactions in the past; 
\item Some parents realized they tended to focus excessively on the intricacy of the storylines crafted by children.;
\end{itemize} 
\\
\cline{2-3}
& Storymaking as Family Meaning Co-constructing
& 
\begin{itemize}[label=--]
\item The storybooks co-created with their children could become part of their family memory archive;
\item Several families indeed used paper cutouts or character tokens of AI-generations at home for making new stories.
\end{itemize} 
\\
\hline
\multirow{3}{*}{Therapists}
& Observing the Strengths and Challenges of Children and Families
& 
\begin{itemize}[label=--]
\item Observe the strengths of the children via storymaking activities and utilize specific techniques to reveal these strengths to both children themselves and their parents while steering the process; 
\item Gain insights into family interaction dynamics and their challenges in communication and relationship through the process and outcome artifacts of the family's joint storymaking.
\end{itemize}  
\\
\cline{2-3}
& Moderating Family Communication through Storymaking
& 
\begin{itemize}[label=--]
\item Facilitate communication through role-playing; 
\item Initiate perspective-taking plays to enhance mutual understanding among family members.
\end{itemize} 
\\
\cline{2-3}
& Offering a Playful and Safe Space
& 
\begin{itemize}[label=--]
\item Offer diverse playful creative tasks from crafting to dramatic play; 
\item Value the importance of affording a safe space where participants feel comfortable while engaging in the creative process and expressing their thoughts
\end{itemize} 
\\
\hline
\end{tabular}
\end{table*}
